# Supplementary material for: iTeach: In the Wild Interactive Teaching for Failure-Driven Adaptation of Robot Perception
Source: arXiv:2410.09072 ancillary file (2026-09-29)
Supplement: Supplementary file 1 [file iTeach_supp.pdf]

# *iTeach*: Interactive Teaching for Robot Perception using Mixed Reality [ Supplementary Material ]

https://irvlutd.github.io/iTeach

**Jishnu Jaykumar P Cole Salvato Vinaya Bomnale Jikai Wang Yu Xiang**

The University of Texas at Dallas

## Contents

**1 IRVLUTD DoorHandle Dataset Construction 2**

**2 Pretraining 4**

**3 Experiment Setup 5**

**4 User Sample Capture Diversity 5**

**5 HoloLens Application 7**

**6 Train and Test Samples 8**

**7 Practical challenges during experiments 9**

# 1 IRVLUTD DoorHandle Dataset Construction

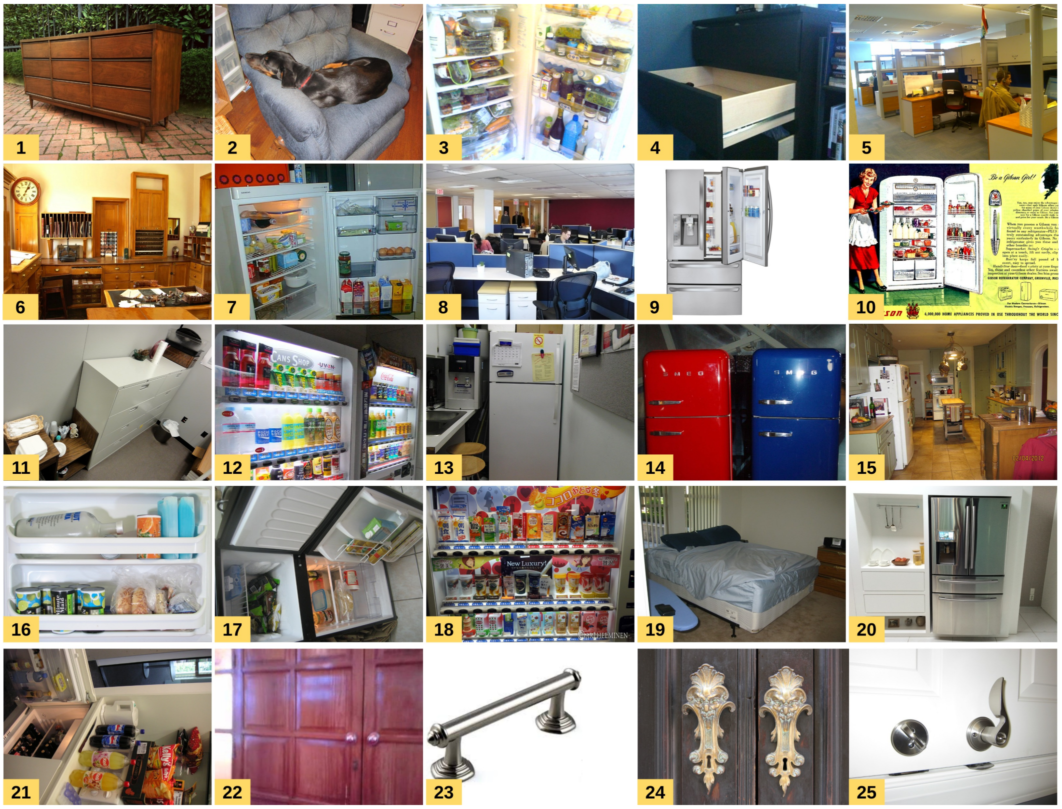


Figure 1: Few samples from the DoorDetect [1] dataset used for pretraining.

The dataset illustrated in Fig. 1 is predominantly composed of kitchen-related images, with a strong emphasis on refrigerators and cabinets. This focus is evident from the high occurrence of refrigerator images (e.g., 3, 7, 9, 12, 14, 16, 17, 18, 20) and broader kitchen scenes (e.g., 6, 15). However, a key limitation of this dataset is its scarcity of images featuring doors and handles—objects critical for robotic applications focused on indoor navigation and manipulation tasks. Only a few images containing doors and handles (e.g., 23, 25) are present, which significantly restricts the dataset's utility for training robust models aimed at detecting and interacting with such objects in real-world environments. The lack of diversity in terms of door types and handle designs, along with the limited number of examples, renders this dataset less effective for robotic tasks that involve complex interactions with doors and handles in a variety of indoor scenarios.

To the best of our knowledge, DoorDetect (DD) [1] is the only dataset specifically designed for door and handle detection. While DD offers a starting point, it falls short in capturing the full complexity and variability of real-world conditions, which are crucial for practical robotic applications. The dataset includes only a limited variety of lighting conditions, occlusions, and environmental features, making it less suitable for real-world scenarios that often involve cluttered spaces, diverse indoor and outdoor settings, unpredictable lighting, narrow pathways, and parallax effects. Additionally, the presence of unwanted appearances, such as people or animals, further complicates the scene for robotic systems.

In response to these shortcomings, we curated a synthetic dataset alongside a modified version of DoorDetect, referred to as DD-Filtered. The original DD dataset contains four classes—door, handle, cabinet door, and refrigerator door. In DD-Filtered, we narrowed the scope by collapsing the cabinet and refrigerator door categories into the general "door" class, resulting in two primary classes: doors

and handles. This filtering was necessary to focus on the objects of primary interest for robotic interaction tasks.

The results of pretraining using both the synthetic and DD-Filtered datasets can be found in Section 2. However, the performance was suboptimal, prompting us to take a more tailored approach to address the gap in real-world applicability.

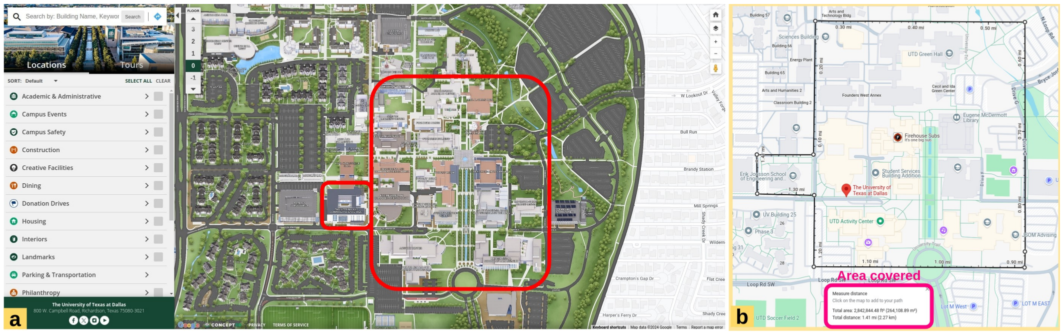


Figure 2: Overview of the total robot navigation area on the UT Dallas campus for the creation of IRVLUTD Door Handle dataset: (a) Map sourced from map.utdallas.edu, (b) Navigation area calculated using Google Maps' measure distance feature.

We developed a new dataset specifically for robotics, which we call the IRVLUTD DoorHandle dataset. Using a Fetch mobile manipulator, we navigated the robot across various locations on the University of Texas at Dallas (UTD) campus, as shown in Fig. 2, capturing images directly from the robot's camera. The choice of using the robot's camera was deliberate, as the view perspective and camera settings play a crucial role in robotic tasks involving object detection and manipulation. The dataset encompasses a wide variety of door and handle types, both indoors and outdoors. These include glass doors, steel handle bars, wooden doors in various colors, doors with posters, fire extinguisher doors (useful in rescue robotics), as well as other distinctive objects like lift doors and vending machine doors. The dataset also features a diverse range of backgrounds—white walls, green, orange, natural outdoor scenes—along with different lighting conditions and door sizes.

In total, we conducted approximately 10-12 hours of robot navigation, resulting in the capture of around 33,000 image samples. After filtering out redundant, blurry, and non-door/handle samples, we retained 1,532 images. While some degree of blurriness remains in the dataset, it was preserved intentionally to simulate the challenges posed by robot navigation during motion. From these 1,532 images, we created two subsets: one containing 524 images and another with 1,008 images. These subsets were used to compare the performance of pretraining models across varying dataset sizes—524 (fewer samples), 1,008 (larger sample set), and the full set of 1,532 samples. The corresponding results are discussed in Section 2.

Furthermore, we created a dedicated test set consisting of images from the 4th floor of the Engineering and Computer Science South (ECSS) building at UTD, disjoint from *train.524* and *train.1008* split. This location served as a testbed for conducting real-world experiments to evaluate the dataset's effectiveness in robotic applications.

All datasets[1], including the IRVLUTD DoorHandle Dataset[2], the DD-Filtered Dataset, and the samples used to create the results table in the main paper, can be found there. We have a PyTorch dataloader for the IRVLUTD DoorHandle Dataset hosted on GitHub[3] and PyPI[4].

[1] https://utdallas.box.com/v/iTeach-Experiment-Datasets
[2] https://utdallas.box.com/v/IRVLUTD-DoorHandle-Dataset
[3] https://github.com/IRVLUTD/IRVLUTDDoorHandleDataset
[4] https://pypi.org/project/IRVLUTDDoorHandleDataset/

## 2 Pretraining

The results of various experiments are summarized in the Table. 1, detailing the performance metrics of different models and datasets. The experiments utilized synthetic data, the DoorDetect dataset, and the IRVLUTD DoorHandle dataset.

We employed the medium-sized variant of YOLOv5 [2] v6.0 for our experiments. The training environment was configured with Python 3.9.19 and PyTorch 2.4.0, running on CUDA 12.1 and utilizing an NVIDIA RTX A5000 GPU with 24 GB of memory. While any YOLO variant could have been selected, we opted for this version due to its availability and comprehensive documentation at the outset of the project.

We began pretraining with a synthetic dataset collected from simulation. As shown in Table 1, and as expected, the simulated data did not generalize well to real-world scenarios. To address this, we filtered the DoorDetect dataset [1], creating what we call DD-Filtered (DDF), which includes only door and handle categories. The original cabinet door and refrigerator door categories were merged into the doors category. When we used a hybrid approach combining the synthetic dataset with DDF, the results improved but did not meet our expectations. Switching to purely DDF led to further improvements, though still not significant. It became clear that pretraining required real-world samples. Thus, we developed the IRVLUTD DoorHandle Dataset, as detailed in Section 1. We observed significant improvements initially when training from scratch using dhyolo-v0 with DDF and train.524 samples. Performance further improved with train.1008, and even more with train.1532. Additionally, using pretrained checkpoints as weight initializers proved beneficial for boosting model performance, as seen in comparisons like exp2 vs. exp3, exp27 vs. exp28 vs. exp29, and exp30 vs. exp31 vs. exp32.

| Experiment | Base | Dataset | Epochs | ckpt-variant | P ↑ | | | R ↑ | | | mAP50 ↑ | | | mAP50-95 ↑ | | |
|---|---|---|---|---|---|---|---|---|---|---|---|---|---|---|---|---|
| | | | | | All | Door | Handle | All | Door | Handle | All | Door | Handle | All | Door | Handle |
| *Using synthetic and DoorDetect [1] Dataset* | | | | | | | | | | | | | | | | |
| sim | ∅ | SYN (50k) | 25 | best & last | 0.356 | 0.315 | 0.398 | 0.412 | 0.526 | 0.298 | 0.293 | 0.359 | 0.228 | 0.127 | 0.182 | 0.0726 |
| hybrid | ∅ | SYN+DDF (4k) | 25 | best & last | 0.582 | 0.553 | 0.611 | 0.423 | 0.428 | 0.418 | 0.398 | 0.402 | 0.393 | 0.161 | 0.193 | 0.129 |
| **real** (†) | ∅ | DDF | 25 | best & last | 0.55 | 0.495 | 0.606 | 0.43 | 0.459 | 0.4 | 0.416 | 0.429 | 0.403 | 0.16 | 0.214 | 0.106 |
| *Using IRVLUTD DoorHandle Dataset* | | | | | | | | | | | | | | | | |
| **exp2** (‡) | † | DDF+524 | 100 | best | 0.837 | 0.919 | 0.756 | 0.674 | **0.745** | 0.604 | 0.732 | 0.824 | 0.641 | 0.478 | 0.688 | 0.267 |
| exp2 | † | DDF+524 | 100 | last | 0.854 | 0.954 | 0.754 | 0.651 | 0.699 | 0.604 | 0.725 | 0.814 | 0.636 | 0.466 | 0.685 | 0.247 |
| exp3 | ∅ | 524 | 100 | best | 0.846 | 0.897 | 0.795 | 0.653 | 0.688 | 0.618 | 0.708 | 0.768 | 0.648 | 0.438 | 0.608 | 0.269 |
| exp3 | ∅ | 524 | 100 | last | 0.874 | 0.936 | 0.811 | 0.636 | 0.675 | 0.596 | 0.708 | 0.775 | 0.64 | 0.434 | 0.611 | 0.257 |
| exp27 | ‡ | 1008 | 100 | best | 0.932 | 0.955 | 0.91 | 0.672 | 0.687 | 0.658 | 0.78 | 0.809 | 0.75 | **0.536** | 0.708 | **0.364** |
| exp27 | ‡ | 1008 | 100 | last | 0.917 | 0.954 | 0.88 | 0.67 | 0.673 | 0.666 | 0.77 | 0.803 | 0.738 | 0.534 | 0.705 | **0.364** |
| exp28 | ∅ | 1008 | 100 | best | 0.916 | 0.946 | 0.886 | 0.64 | 0.637 | 0.644 | 0.736 | 0.761 | 0.712 | 0.459 | 0.607 | 0.311 |
| exp28 | ∅ | 1008 | 100 | last | 0.91 | 0.94 | 0.88 | 0.645 | 0.65 | 0.64 | 0.737 | 0.764 | 0.71 | 0.459 | 0.61 | 0.308 |
| exp29 | † | 1008 | 100 | best | 0.922 | 0.953 | 0.89 | 0.676 | 0.678 | 0.675 | 0.764 | 0.799 | 0.729 | 0.515 | 0.682 | 0.349 |
| exp29 | † | 1008 | 100 | last | 0.926 | 0.942 | 0.91 | 0.66 | 0.655 | 0.664 | 0.753 | 0.789 | 0.718 | 0.512 | 0.686 | 0.338 |
| exp30 | ‡ | 1532 | 100 | best | 0.93 | **0.976** | 0.884 | 0.676 | 0.688 | 0.664 | 0.785 | 0.825 | 0.744 | 0.534 | 0.706 | 0.362 |
| exp30 | ‡ | 1532 | 100 | last | 0.909 | 0.96 | 0.858 | 0.695 | 0.714 | **0.714** | **0.786** | 0.821 | **0.752** | 0.531 | 0.718 | 0.343 |
| exp31 | † | 1532 | 100 | best | 0.918 | 0.968 | 0.869 | **0.708** | 0.728 | 0.687 | 0.781 | **0.831** | 0.731 | 0.532 | **0.723** | 0.341 |
| exp31 | † | 1532 | 100 | last | 0.914 | 0.963 | 0.866 | 0.681 | 0.699 | 0.662 | 0.77 | 0.827 | 0.714 | 0.529 | 0.719 | 0.339 |
| exp32 | ∅ | 1532 | 100 | best | 0.904 | 0.946 | 0.861 | 0.657 | 0.669 | 0.644 | 0.74 | 0.778 | 0.703 | 0.47 | 0.629 | 0.31 |
| exp32 | ∅ | 1532 | 100 | last | **0.941** | 0.953 | **0.93** | 0.651 | 0.659 | 0.644 | 0.744 | 0.781 | 0.707 | 0.47 | 0.638 | 0.301 |

Table 1: The metric values are presented within the [0-1] range. **SYN** refers to the Synthetic dataset, **DDF** denotes the DD-Filtered dataset, **524** corresponds to train.524, **1008** to train.1008, and **1532** to train.1532. The symbol ∅ indicates models trained from scratch, using random weight initialization. **†:** refers to dhyolo-v0, while **‡:** denotes dhyolo-v1. The terms **best** and **last** represent the best and final epoch model checkpoints obatined at the end of each training session, respectively.

We chose not to release the synthetic dataset because it did not effectively enhance model performance. Instead, we have made the **DDF** variant of the DoorDetect [1] dataset available, along with the necessary model checkpoints. For the fine-tuning process, we selected the **dhyolo-v1**‡ model as our starting checkpoint. This decision was made to ensure we had a model that balanced performance; it needed to be good enough to provide useful feedback but not so high-performing that it would lack the faulty samples we needed for training. The core idea behind the iTeach framework is to utilize incorrect predictions as learning signals for improving the model. By focusing on these errors, we aim to refine the model's accuracy, allowing it to learn from its mistakes and adapt better to complex real-world situations. This process ultimately enhances the model's overall reliability and effectiveness in practical applications. The pretrained checkpoints, including both the best and the last versions, trained on the IRVLUTD DoorHandle Dataset, can be accessed at `https://utdallas.box.com/v/DHYOLO-Pretrained-Checkpoints`.

## 3 Experiment Setup

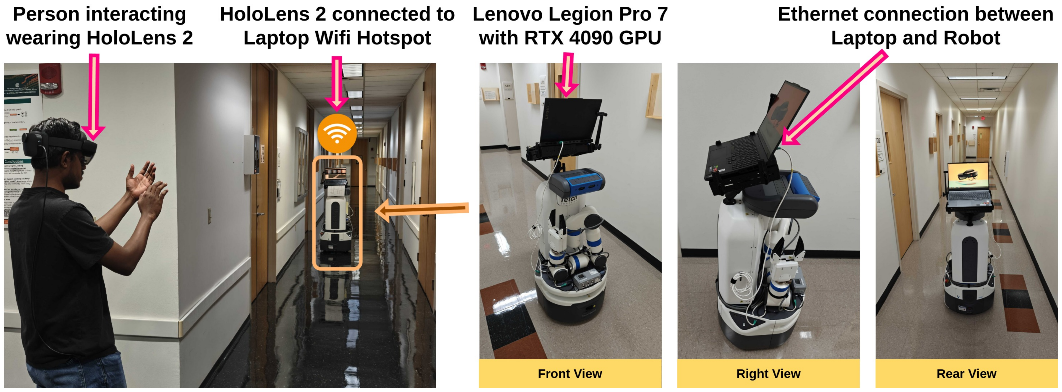


Figure 3: Our experimental setup included a Fetch mobile robot, a HoloLens 2 device, a Lenovo Legion Pro 7 laptop equipped with an RTX 4090 GPU, and a human instructor. The laptop environment is configured with Python 3.8.10 and PyTorch 2.4.0, utilizing CUDA 12.1 and an NVIDIA GeForce RTX 4090 Laptop GPU, which has approximately 16 GB of memory.

Our setup consists of a mobile Fetch robot, a laptop mounted on top of the robot, and a HoloLens worn by the teacher (human operator). As depicted in Fig. 3, the system is divided into two subnetworks: one between the laptop and HoloLens, established via a Wi-Fi hotspot hosted by the laptop, and the other between the robot and the laptop using an Ethernet connection for fast data transfer. Model training and data storage are managed on the laptop, with the ROS server running on the robot. Communication between the HoloLens and robot is facilitated by the ROS TCP endpoint connector[5], while the laptop and robot communicate using the standard ROS framework.

## 4 User Sample Capture Diversity

As illustrated in Fig. 4a, we outline several potential scenarios where mispredicted samples could be collected. The specific scenarios may vary based on the human assisting with the data collection process. The effectiveness of **iTeach** is heavily dependent on human judgment in this aspect.

**False Positives and False Negatives.** These represent instances where the system incorrectly classifies either non-door/handle objects as doors/handles (false positives) or fails to detect an actual door/handle (false negatives). In robotic systems, false positives could include items like cabinets or walls being misclassified as doors, while false negatives might occur in complex environments where the door or handle blends into the background or is partially obscured. These errors could lead to inefficiencies in tasks like door navigation and manipulation. Minimizing these errors is critical for improving detection reliability, especially in environments with high variability.

**Scaled View and Narrow Path.** This scenario refers to varying object scales due to changes in distance between the robot and the door/handle, as well as constrained spaces where navigation is challenging. Scaled views may occur when the robot approaches a door from different distances, affecting the size and clarity of the object in the frame. Narrow path scenarios present additional challenges for navigation, as the robot may need to adjust its position carefully to detect and interact with objects in tight spaces. Systems trained with diverse scale examples are better equipped to handle varying object sizes and maintain detection accuracy across different distances. Handling narrow paths is crucial for improving real-world navigation performance.

**Occlusion and Person in View.** This refers to situations where parts of the door or handle are blocked (occluded) by other objects, or when a person is present in the scene, potentially interfering with the robot's ability to focus on the target objects. Occlusion, whether caused by furniture, other doors,

[5]https://github.com/Unity-Technologies/ROS-TCP-Connector

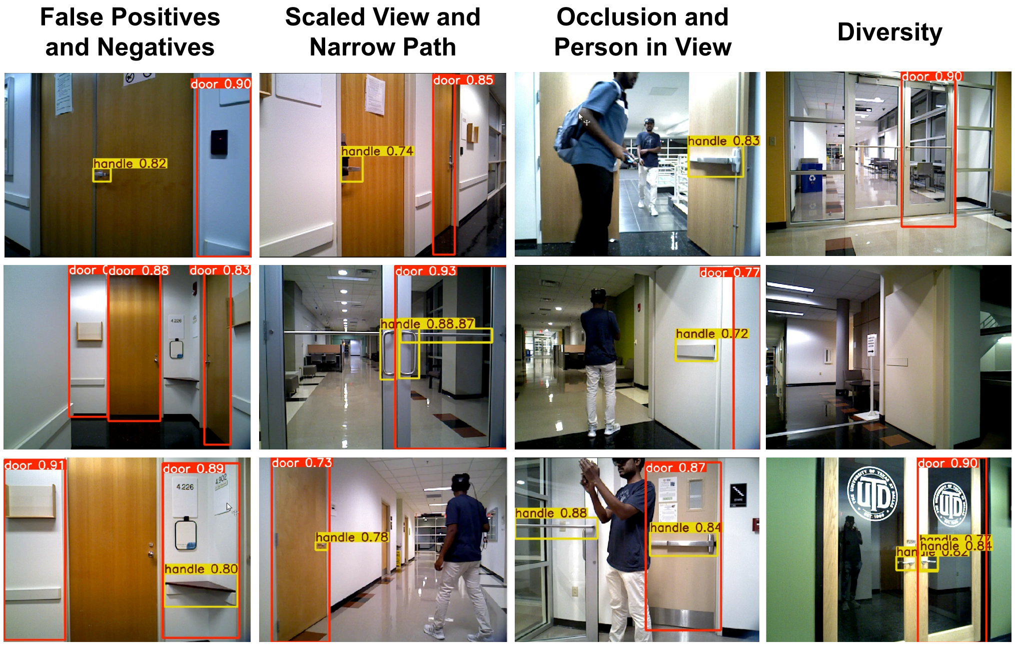


(a) Sample collection via robot navigation at different places.

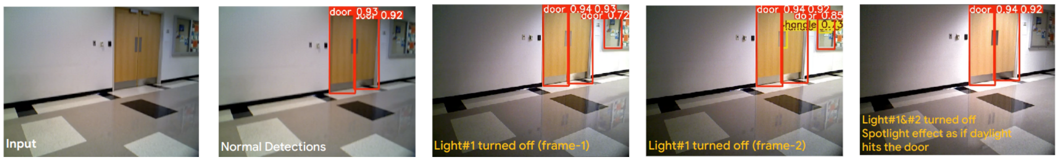


(b) Different samples collected from the same location under varying lighting conditions suggest that multiple samples can be obtained from a single site.

Figure 4: Sample collection scenarios for fine-tuning. Images are captured from the robot camera.

or even people, adds complexity to object detection. The presence of humans introduces dynamic elements that require the robot to distinguish between relevant and irrelevant objects for its task. This is particularly challenging in shared environments, like offices or homes. Robust detection models need to generalize well under occlusion and clutter, ensuring that the robot can reliably detect and interact with doors and handles even in crowded spaces.

**Diversity in Lighting and Object Appearance.** Variations in lighting conditions (e.g., bright sunlight, shadows, indoor lighting) and the appearance of doors and handles (e.g., color, material, design) contribute to the diversity of test scenarios. Different lighting conditions can significantly alter the appearance of doors and handles, making detection more difficult in low light or shadowed areas. Additionally, the diversity in door/handle materials—such as glass doors, wooden doors with painted finishes, or metallic handles—requires the system to adapt to varying textures and colors. Accounting for this diversity is essential for real-world deployment, where lighting and object appearance may change frequently. A well-trained model should handle both high-contrast and low-light scenarios with minimal degradation in performance.

**Indoor and Outdoor Varieties.** This scenario highlights the difference between indoor and outdoor environments, which bring distinct challenges in terms of lighting, object variety, and potential distractions. Indoor environments, like hallways or office spaces, generally provide more controlled lighting but may introduce clutter and tight spaces. Outdoor settings, on the other hand, expose the system to natural elements, such as sunlight, shadows, and potentially unpredictable backgrounds (e.g., trees, other buildings). The transition between these environments poses additional complexity for the system. A system that performs well across both indoor and outdoor scenarios is vital for applications in mixed environments, where the robot may have to transition seamlessly between them.

**Unwanted Appearances.** This scenario refers to distractions or obstacles in the robot's field of view, such as people, pets, or irrelevant objects, that could confuse the detection system. The presence of moving objects or irrelevant items (like animals or people) in the environment could result in misclassification or distract the system from its primary task. Handling these distractions effectively is crucial for reliable performance in public spaces or homes. By training models on datasets that account for these distractions, we can improve the robot's ability to focus on doors and handles even in dynamic, unpredictable environments.

# 5 HoloLens Application

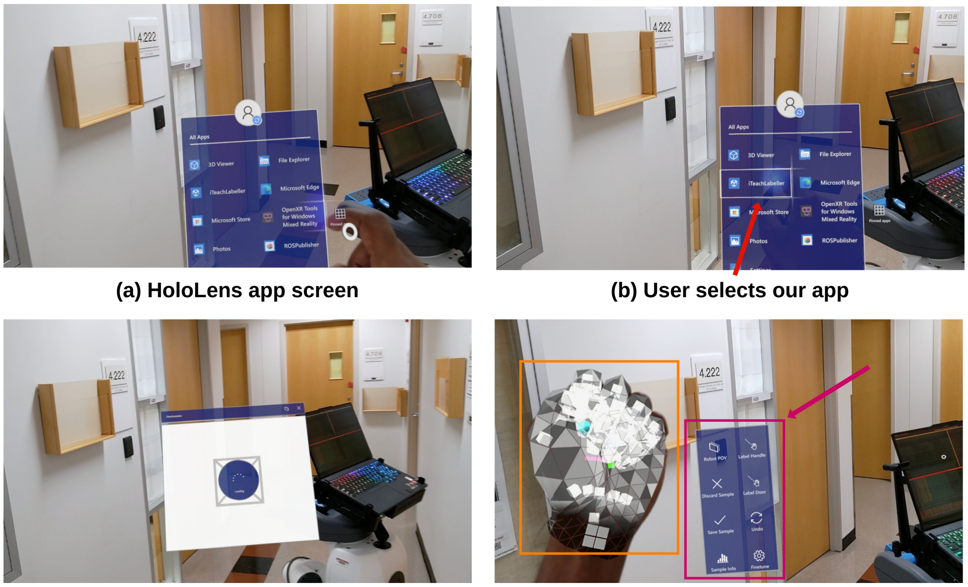

**(a) HoloLens app screen** **(b) User selects our app**

**(c) Our app starts to load** **(d) Our app maps user's closed left palm gesture and the main menu pops up.**

Figure 5: The user interface flow of our labeling app from the startup phase to the main menu.

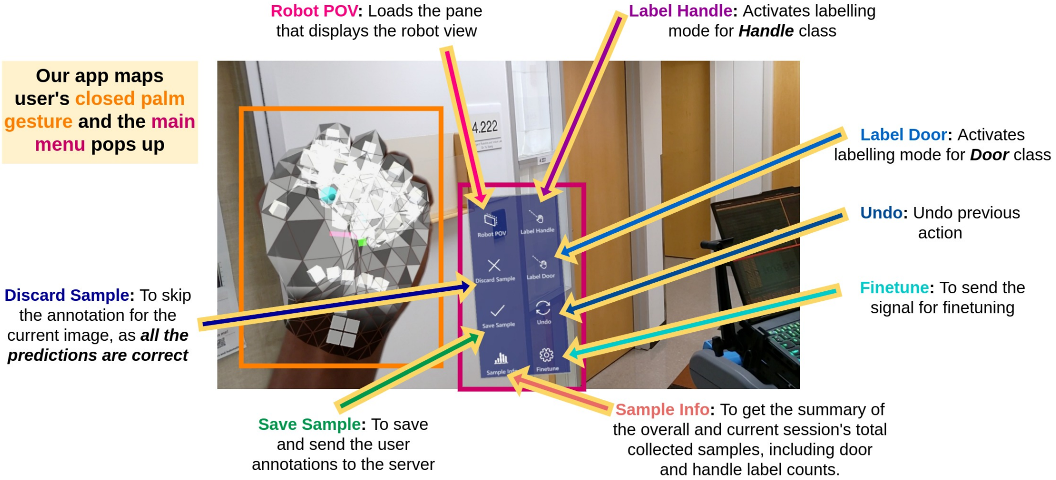


Figure 6: Description of the main menu options in the *iTeachlabeller* app.

[5] A build is available at `https://utdallas.box.com/v/iTeachLabellerApp`.

# 6 Train and Test Samples

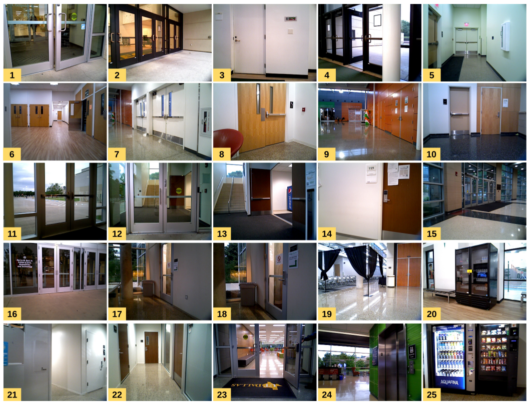

(a) train.524 split.

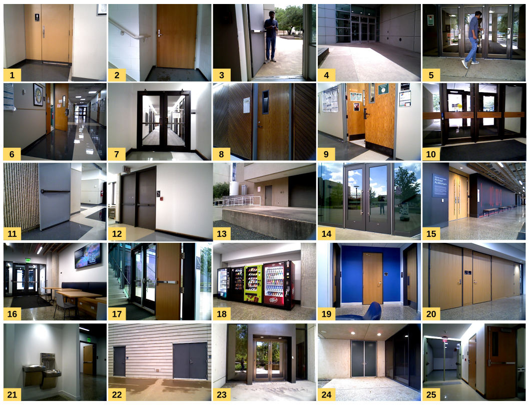

(b) train.1008 split.

Figure 7: Comparison of the train.524 and train.1008 splits, showcasing a variety of doors and handles with different scales, backgrounds, lighting conditions, occlusion, and both indoor and outdoor environments.

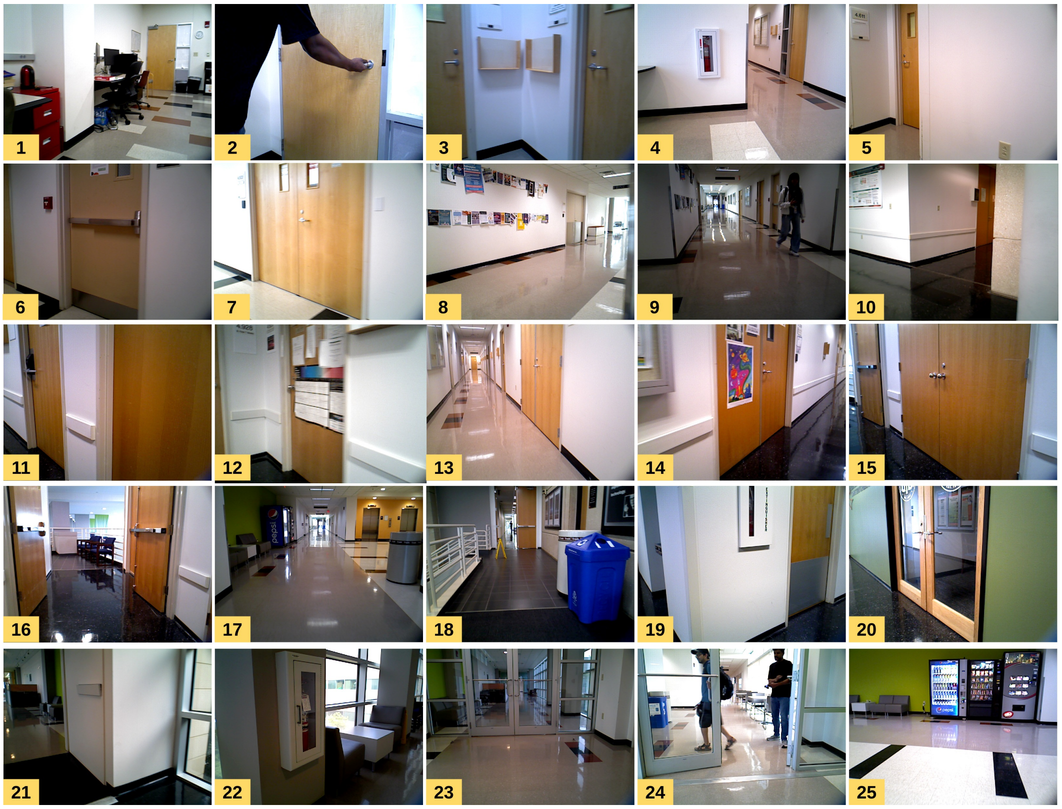

Figure 8: Few samples from the test.256 split showing different varieties of door handle test scenarios. Location: UTD-ECSS-Floor-4.

# 7 Practical challenges during experiments

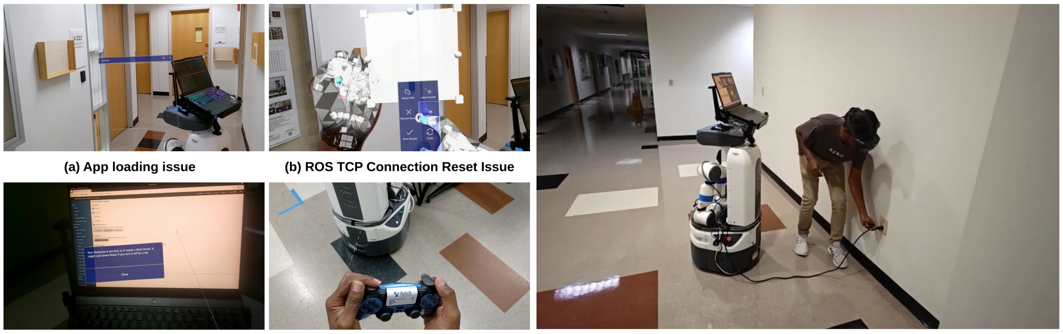

(a) App loading issue (b) ROS TCP Connection Reset Issue (c) HoloLens Overheating (d) Fetch Controller Bluetooth Connection Reset/Lost (e) Laptop battery discharge

Figure 9: Challenges faced in the real world during the execution of our experiments.

Our system consists of several open-source modules, including ROS-TCP-Connector, Unity, and the Windows SDK for HoloLens 2 app development. We heavily depend on their stability for optimal functionality. The challenges we faced primarily arise from these modules, as depicted in the figure. The laptop's battery drains as it runs multiple modules, manages a mobile hotspot, and operates the GPU; this battery drain is a natural consequence. A simple UPS could resolve this issue, but for extended sessions, users must switch to charging mode. However, it's feasible to collect diverse samples while charging, as demonstrated in the demo video and Fig. 4b.

Additionally, we encountered issues during the HoloLens 2 app build process. While the app works flawlessly in simulation, building it relies significantly on configurations in Visual Studio, Unity, and the HoloLens UWP version. Therefore, it's important to set up a standalone development environment, or you can utilize our provided app build. The fetch robot's battery lasts several hours, so that won't be a concern. For the HoloLens, we use a power bank to ensure it doesn't run out of battery, which can conveniently fit in the user's pocket with a wire attached.

Another challenge we faced is the HoloLens overheating, which is also a natural occurrence. To address this, short breaks are necessary, allowing users to rest while preventing overheating. Each of these challenges comes with corresponding benefits that enhance the overall use case of the system. In summary, these challenges are manageable, as demonstrated by our fully functional system.

## References


[1] M. Arduengo, C. Torras, and L. Sentis. Robust and adaptive door operation with a mobile robot. *Intelligent Service Robotics*, May 2021. ISSN 1861-2784. doi:10.1007/s11370-021-00366-7. URL http://dx.doi.org/10.1007/s11370-021-00366-7. 2, 4

[2] G. Jocher. ultralytics/yolov5: v3.1 - Bug Fixes and Performance Improvements. https://github.com/ultralytics/yolov5, Oct. 2020. URL https://doi.org/10.5281/zenodo.4154370. 4
